# Supplementary material for: Two-dimensional partitioned square ice confined in graphene/graphite nanocapillaries
Source: arXiv:2204.03198 source file (2022-04-07)
Supplement: Supplementary file 1 [file Supplementary_Material.pdf]

## Supplementary Material

# Two-Dimensional Partitioned Square Ice Confined in Graphene/Graphite Nanocapillaries

*Zhen Zeng*[1], *Tianyou Wang*[1]*, *Rui Chen*[2], *Mengshan Suo*[1], *Kai Sun*[1],

*Panagiotis E. Theodorakis*[3], *and Zhizhao Che*[1]*

[1]State Key Laboratory of Engines, Tianjin University, Tianjin 300072, China

[2]Department of Aeronautical and Automotive Engineering, Loughborough University, Loughborough LE11 3TU, United Kingdom

[3]Institute of Physics, Polish Academy of Sciences, Al. Lotników 32/46, 02-668 Warsaw, Poland

*Corresponding Authors.

*Email address: wangtianyou@tju.edu.cn (Tianyou Wang); chezhizhao@tju.edu.cn (Zhizhao Che)

Movie S1. A video clip of the transformation from the partitioned SI structure to the homogeneous SI structure occurs in the pressurization process corresponding to Figure S2. The red beads represent oxygen atoms and the cyan beads represent hydrogen atoms.

Movie S2. A video clip of the constrained water during the pressurization process corresponding to Figure 3(a). The red beads represent oxygen atoms and the cyan beads represent hydrogen atoms.

Movie S3. A video clip of the constrained water during the heating process corresponding to Figure 3(b). The red beads represent oxygen atoms and the cyan beads represent hydrogen atoms.

Movie S4. A video clip of the typical scenario of square ice formation for $n = 1$ corresponding to Figure 6(b), in which the region with different icing orientation disappears. The red beads represent oxygen atoms and the cyan beads represent hydrogen atoms.

Movie S5. A video clip of the typical scenario of square ice formation for $n = 2$ corresponding to Figure 7(b), in which the region with different icing orientation enlarges and stabilizes. The red beads represent oxygen atoms and the cyan beads represent hydrogen atoms.

Movie S6. A video clip of the typical scenario of square ice formation for $n = 2$ corresponding to Figure 7(c), in which more than two regions have different icing orientations. The red beads represent oxygen atoms and the cyan beads represent hydrogen atoms.

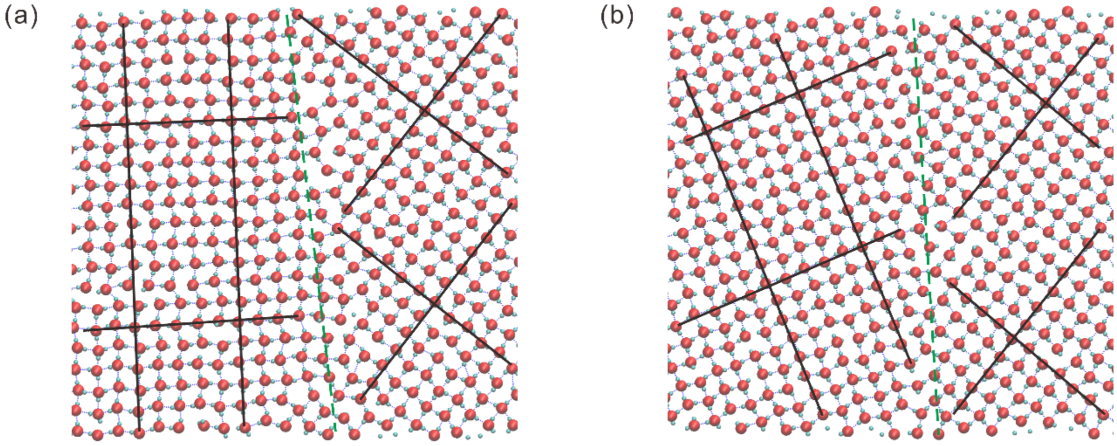


Figure S1 Top views of the simulation results with different graphene stackings. (a) ABA stacking. (b) AAA stacking.

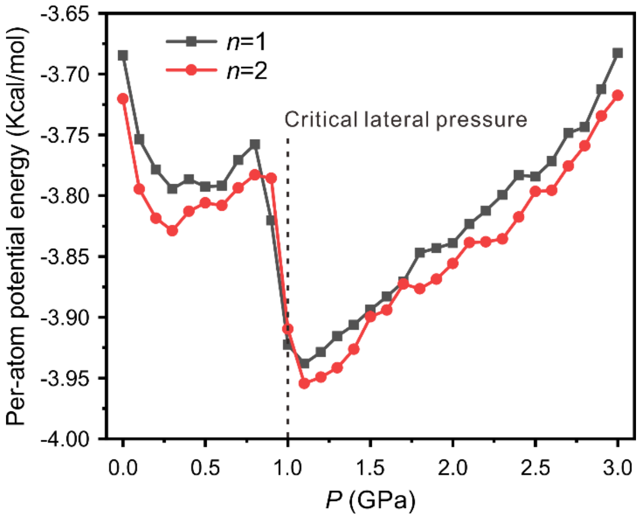


Figure S2 Lateral pressure dependence of the potential energy per molecule of bilayer ice ($h$ = 9.0 Å, $T$ = 298 K). Black and red lines indicate the potential energy per molecule for $n$ = 1 and $n$ = 2, respectively.

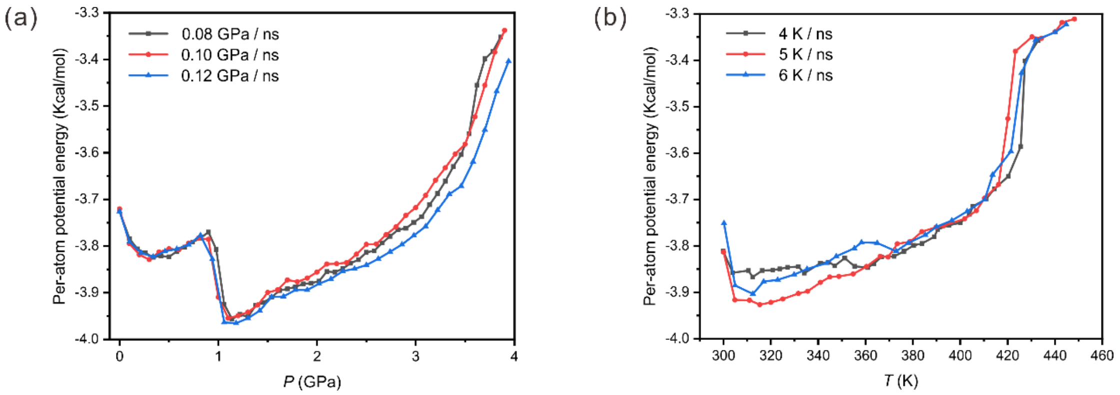


Figure S3 Variation of the potential energy of the confined water during the pressurization and heating process. (a) At different pressurization rates (0.08 GPa/ns, 0.10 GPa/ns, and 0.12 GPa/ns). (b) At different heating rates (4 K/ns, 5 K/ns, and 6 K/ns).

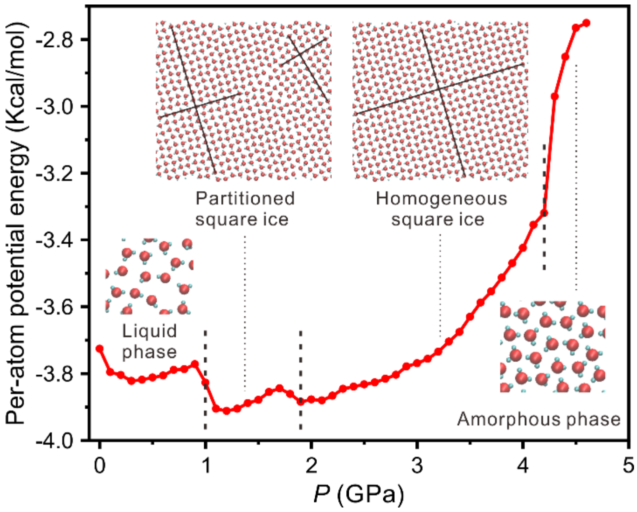


Figure S4 Variation of the potential energy of the constrained water during the pressurization process. The red beads represent oxygen atoms, the cyan beads represent hydrogen atoms, the blue dashed lines represent hydrogen bonds and the black solid line is a guide of the icing direction to the eye.

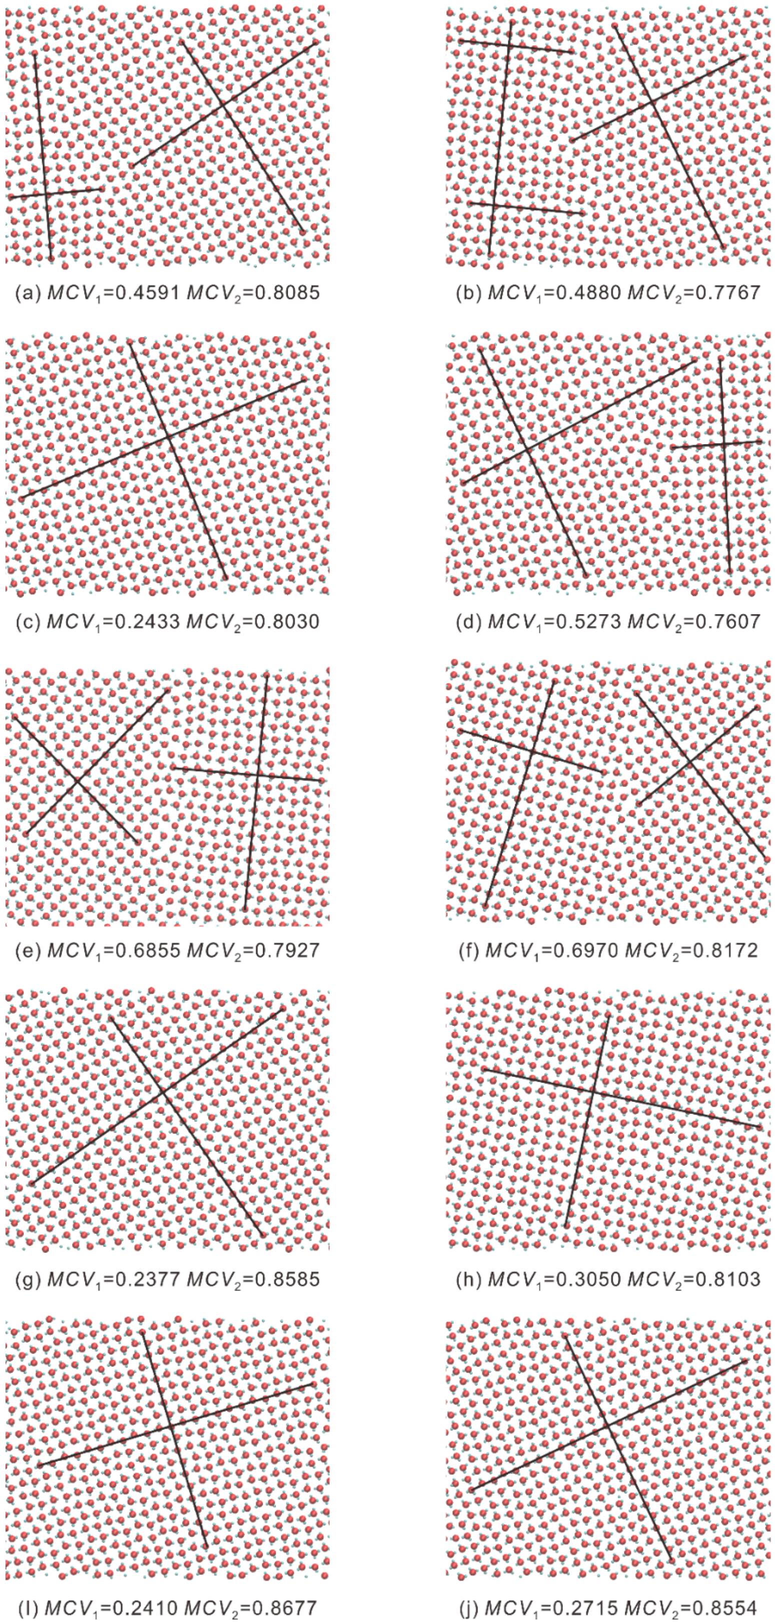


Figure S5 More partitioned square icing patterns for $n$ = 2. Each figure represents a repeated simulation with different initial velocity distribution of water molecules while keeping the other settings identical. The red beads represent oxygen atoms and the cyan beads represent hydrogen atoms.

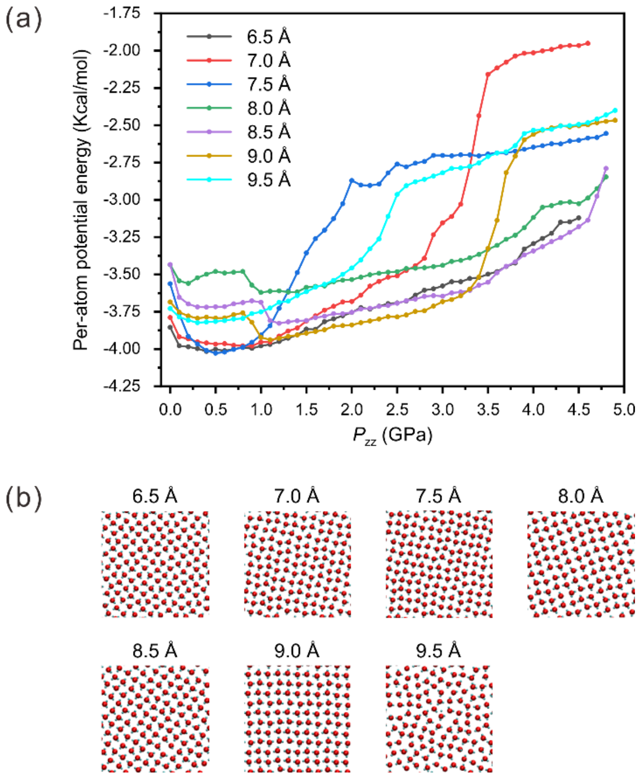


Figure S6 (a) Lateral pressure dependence of the potential energy per molecule of confined water with different widths of the nanocapillaries ($h$ = 6.5 Å, 7.0 Å, 7.5 Å, 8.0 Å, 8.5 Å, 9.0 Å, and 9.5 Å). (b) The 2D structures under different nanocapillaries ($P_{zz}$ = 1.1 GPa).
